# Supplementary material for: A Graduated Filter Method for Large Scale Robust Estimation
Source: arXiv:2003.09080 source file (2020-03-20)
Supplement: Supplementary file 1 [file algo_filter.tex]

\begin{algorithm}[ht]\centering
\caption{Optimization with Filter Method}
\label{alg:filter}                         
\begin{algorithmic}[1]                   
	\REQUIRE Initial solution $\bx^0$, filter margin $\alpha$, \texttt{max\_iter}
	\STATE  Initialization: $t \leftarrow 0$, $\cF \leftarrow \emptyset$ , $\bbF \leftarrow \emptyset$
	\WHILE{\texttt{true} and $t<$ \texttt{max\_iter}}
	    \IF{$\bx^t$ is stationary}
	        \STATE break;
	    \ENDIF
	    \STATE $\tilde{f}\leftarrow f_t - \alpha h_t$;  $\tilde{h} \leftarrow h_t - \alpha h_t$
	    %\STATE $F_{t+1} \leftarrow (\tilde{f},\tilde{h})$
	    \STATE $\cF \leftarrow \cF \cup \{(\tilde{f}, \tilde{h})\}$
	    \STATE $\bF_{t+1} \leftarrow \{\bx | f(\bx) \ge \tilde{f}, h(\bx) \ge \tilde{h} \}$ %Forbidden region
	    \STATE $\bbF \leftarrow \bbF \cup \bF_{t+1}$
	    \STATE Compute $\bx^{t+1} \notin \bbF$ \label{alg:line:compute_x} (Sec.~\ref{sec:coop_step} and~\ref{sec:restore_step})
	    \IF{$f(\bx^{t+1}) < f(\bx^{t})$}
	        \STATE $\cF \leftarrow \cF \setminus \{(\tilde{f}, \tilde{h})\}$; $\bbF \leftarrow \bbF \setminus \bF_{t+1}$
	    \ENDIF
	    \STATE $t \leftarrow t + 1$
	\ENDWHILE
	\RETURN $\bx^t$
\end{algorithmic}
\end{algorithm}
