# Supplementary material for: A Graduated Filter Method for Large Scale Robust Estimation
Source: arXiv:2003.09080 source file (2020-03-20)
Supplement: Supplementary file 2 [file table_inliers.tex]

\begin{table}[ht]
\centering
\resizebox{1.0\columnwidth}{!}{
\begin{tabular}{|l|l|l|l|l|l|}
\hline
           &  IRLS    & M-HQ   & GNC   & MOO     & ASKER \\ \hline
Ladybug-49 &  80.4    &  \textbf{82.3}  & 82.1  & 81.9    & \textbf{82.3}  \\ \hline
Trafalgar-21 &  50.9    &  69.0  & 68.3  & 68.8    & \textbf{69.10}  \\ \hline
Trafalgar-201 &  66.31    &  69.2  & 69.1  & 68.8    & \textbf{69.33}  \\ \hline
Trafalgar-225 &  67.05    &  69.8  & 69.9  & \textbf{70.01}    & \textbf{70.01}  \\ \hline

\end{tabular}
}
\caption{Inlier percentage achieved by the methods}
\label{table:results_inliers}
\end{table}
